# Supplementary material for: Detecting Gang-Involved Escalation on Social Media Using Context
Source: arXiv:1809.03632 source file (2018-09-10)
Supplement: Supplementary file 1 [file emnlp2018.tex]

%
% File emnlp2018.tex
%
%% Based on the style files for EMNLP 2018, which were
%% Based on the style files for ACL 2018, which were
%% Based on the style files for ACL-2015, with some improvements
%%  taken from the NAACL-2016 style
%% Based on the style files for ACL-2014, which were, in turn,
%% based on ACL-2013, ACL-2012, ACL-2011, ACL-2010, ACL-IJCNLP-2009,
%% EACL-2009, IJCNLP-2008...
%% Based on the style files for EACL 2006 by 
%%e.agirre@ehu.es or Sergi.Balari@uab.es
%% and that of ACL 08 by Joakim Nivre and Noah Smith

\documentclass[11pt,a4paper]{article}
\usepackage[hyperref]{emnlp2018}
\usepackage{times}
\usepackage{latexsym}

\usepackage{url}

%\aclfinalcopy % Uncomment this line for the final submission
%\def\aclpaperid{***} %  Enter the acl Paper ID here

%\setlength\titlebox{5cm}
% You can expand the titlebox if you need extra space
% to show all the authors. Please do not make the titlebox
% smaller than 5cm (the original size); we will check this
% in the camera-ready version and ask you to change it back.

\newcommand\BibTeX{B{\sc ib}\TeX}
\newcommand\confname{EMNLP 2018}
\newcommand\conforg{SIGDAT}

\title{Instructions for \confname{} Proceedings}

\author{First Author \\
  Affiliation / Address line 1 \\
  Affiliation / Address line 2 \\
  Affiliation / Address line 3 \\
  {\tt email@domain} \\\And
  Second Author \\
  Affiliation / Address line 1 \\
  Affiliation / Address line 2 \\
  Affiliation / Address line 3 \\
  {\tt email@domain} \\}

\date{}

\begin{document}
\maketitle
\begin{abstract}
  This document contains the instructions for preparing a camera-ready
  manuscript for the proceedings of \confname{}. The document itself
  conforms to its own specifications, and is therefore an example of
  what your manuscript should look like. These instructions should be
  used for both papers submitted for review and for final versions of
  accepted papers.  Authors are asked to conform to all the directions
  reported in this document.
\end{abstract}

\section{Credits}

This document has been adapted from the instructions for earlier ACL
and NAACL proceedings. It represents a recent build from
\url{https://github.com/acl-org/acl-pub}, with modifications by Micha
Elsner and Preethi Raghavan, based on the NAACL 2018 instructions by
Margaret Michell and Stephanie Lukin, 2017/2018 (NA)ACL bibtex
suggestions from Jason Eisner, ACL 2017 by Dan Gildea and Min-Yen Kan,
NAACL 2017 by Margaret Mitchell, ACL 2012 by Maggie Li and Michael
White, those from ACL 2010 by Jing-Shing Chang and Philipp Koehn,
those for ACL 2008 by Johanna D. Moore, Simone Teufel, James Allan,
and Sadaoki Furui, those for ACL 2005 by Hwee Tou Ng and Kemal
Oflazer, those for ACL 2002 by Eugene Charniak and Dekang Lin, and
earlier ACL and EACL formats.  Those versions were written by several
people, including John Chen, Henry S. Thompson and Donald
Walker. Additional elements were taken from the formatting
instructions of the {\em International Joint Conference on Artificial
  Intelligence} and the \emph{Conference on Computer Vision and
  Pattern Recognition}.

\section{Introduction}

The following instructions are directed to authors of papers submitted
to \confname{} or accepted for publication in its proceedings. All
authors are required to adhere to these specifications. Authors are
required to provide a Portable Document Format (PDF) version of their
papers. \textbf{The proceedings are designed for printing on A4
paper.}

\section{General Instructions}

Manuscripts must be in two-column format.  Exceptions to the
two-column format include the title, authors' names and complete
addresses, which must be centered at the top of the first page, and
any full-width figures or tables (see the guidelines in
Subsection~\ref{ssec:first}). {\bf Type single-spaced.}  Start all
pages directly under the top margin. See the guidelines later
regarding formatting the first page.  The manuscript should be
printed single-sided and its length
should not exceed the maximum page limit described in Section~\ref{sec:length}.
Pages are numbered for  initial submission. However, {\bf do not number the pages in the camera-ready version}.

By uncommenting {\small\verb|\aclfinalcopy|} at the top of this 
 document, it will compile to produce an example of the camera-ready formatting; by leaving it commented out, the document will be anonymized for initial submission.  When you first create your submission on softconf, please fill in your submitted paper ID where {\small\verb|***|} appears in the {\small\verb|\def\aclpaperid{***}|} definition at the top.

The review process is double-blind, so do not include any author information (names, addresses) when submitting a paper for review.  
However, you should maintain space for names and addresses so that they will fit in the final (accepted) version.  The \confname{} \LaTeX\ style will create a titlebox space of 2.5in for you when {\small\verb|\aclfinalcopy|} is commented out.  

The author list for submissions should include all (and only) individuals who made substantial contributions to the work presented. Each author listed on a submission to \confname{} will be notified of submissions, revisions and the final decision. No authors may be added to or removed from submissions to \confname{} after the submission deadline.

\subsection{The Ruler}
The \confname{} style defines a printed ruler which should be presented in the
version submitted for review.  The ruler is provided in order that
reviewers may comment on particular lines in the paper without
circumlocution.  If you are preparing a document without the provided
style files, please arrange for an equivalent ruler to
appear on the final output pages.  The presence or absence of the ruler
should not change the appearance of any other content on the page.  The
camera ready copy should not contain a ruler. (\LaTeX\ users may uncomment the {\small\verb|\aclfinalcopy|} command in the document preamble.)  

Reviewers: note that the ruler measurements do not align well with
lines in the paper -- this turns out to be very difficult to do well
when the paper contains many figures and equations, and, when done,
looks ugly. In most cases one would expect that the approximate
location will be adequate, although you can also use fractional
references ({\em e.g.}, the first paragraph on this page ends at mark $108.5$).

\subsection{Electronically-available resources}

\conforg{} provides this description in \LaTeX2e{} ({\small\tt
  emnlp2018.tex}) and PDF format ({\small\tt emnlp2018.pdf}), along
with the \LaTeX2e{} style file used to format it ({\small\tt
  emnlp2018.sty}) and an ACL bibliography style ({\small\tt
  acl\_natbib\_nourl.bst}) and example bibliography ({\small\tt
  emnlp2018.bib}).  These files are all available at
\url{http://emnlp2018.org/downloads/emnlp18-latex.zip}; a Microsoft
Word template file ({\small\tt emnlp18-word.docx}) and example
submission pdf ({\small\tt emnlp18-word.pdf}) is available at
\url{http://emnlp2018.org/downloads/emnlp18-word.zip}.  We strongly
recommend the use of these style files, which have been appropriately
tailored for the \confname{} proceedings.

\subsection{Format of Electronic Manuscript}
\label{sect:pdf}

For the production of the electronic manuscript you must use Adobe's
Portable Document Format (PDF). PDF files are usually produced from
\LaTeX\ using the \textit{pdflatex} command. If your version of
\LaTeX\ produces Postscript files, you can convert these into PDF
using \textit{ps2pdf} or \textit{dvipdf}. On Windows, you can also use
Adobe Distiller to generate PDF.

Please make sure that your PDF file includes all the necessary fonts
(especially tree diagrams, symbols, and fonts with Asian
characters). When you print or create the PDF file, there is usually
an option in your printer setup to include none, all or just
non-standard fonts.  Please make sure that you select the option of
including ALL the fonts. \textbf{Before sending it, test your PDF by
  printing it from a computer different from the one where it was
  created.} Moreover, some word processors may generate very large PDF
files, where each page is rendered as an image. Such images may
reproduce poorly. In this case, try alternative ways to obtain the
PDF. One way on some systems is to install a driver for a postscript
printer, send your document to the printer specifying ``Output to a
file'', then convert the file to PDF.

It is of utmost importance to specify the \textbf{A4 format} (21 cm
x 29.7 cm) when formatting the paper. When working with
{\tt dvips}, for instance, one should specify {\tt -t a4}.
Or using the command \verb|\special{papersize=210mm,297mm}| in the latex
preamble (directly below the \verb|\usepackage| commands). Then using 
{\tt dvipdf} and/or {\tt pdflatex} which would make it easier for some.

Print-outs of the PDF file on A4 paper should be identical to the
hardcopy version. If you cannot meet the above requirements about the
production of your electronic submission, please contact the
publication chairs as soon as possible.

\subsection{Layout}
\label{ssec:layout}

Format manuscripts two columns to a page, in the manner these
instructions are formatted. The exact dimensions for a page on A4
paper are:

\begin{itemize}
\item Left and right margins: 2.5 cm
\item Top margin: 2.5 cm
\item Bottom margin: 2.5 cm
\item Column width: 7.7 cm
\item Column height: 24.7 cm
\item Gap between columns: 0.6 cm
\end{itemize}

\noindent Papers should not be submitted on any other paper size.
 If you cannot meet the above requirements about the production of 
 your electronic submission, please contact the publication chairs 
 above as soon as possible.

\subsection{Fonts}

For reasons of uniformity, Adobe's {\bf Times Roman} font should be
used. In \LaTeX2e{} this is accomplished by putting

\begin{quote}
\begin{verbatim}
\usepackage{times}
\usepackage{latexsym}
\end{verbatim}
\end{quote}
in the preamble. If Times Roman is unavailable, use {\bf Computer
  Modern Roman} (\LaTeX2e{}'s default).  Note that the latter is about
  10\% less dense than Adobe's Times Roman font.

\begin{table}[t!]
\begin{center}
\begin{tabular}{|l|rl|}
\hline \bf Type of Text & \bf Font Size & \bf Style \\ \hline
paper title & 15 pt & bold \\
author names & 12 pt & bold \\
author affiliation & 12 pt & \\
the word ``Abstract'' & 12 pt & bold \\
section titles & 12 pt & bold \\
document text & 11 pt  &\\
captions & 10 pt & \\
abstract text & 10 pt & \\
bibliography & 10 pt & \\
footnotes & 9 pt & \\
\hline
\end{tabular}
\end{center}
\caption{\label{font-table} Font guide. }
\end{table}

\subsection{The First Page}
\label{ssec:first}

Center the title, author's name(s) and affiliation(s) across both
columns. Do not use footnotes for affiliations. Do not include the
paper ID number assigned during the submission process. Use the
two-column format only when you begin the abstract.

{\bf Title}: Place the title centered at the top of the first page, in
a 15-point bold font. (For a complete guide to font sizes and styles,
see Table~\ref{font-table}) Long titles should be typed on two lines
without a blank line intervening. Approximately, put the title at 2.5
cm from the top of the page, followed by a blank line, then the
author's names(s), and the affiliation on the following line. Do not
use only initials for given names (middle initials are allowed). Do
not format surnames in all capitals ({\em e.g.}, use ``Mitchell'' not
``MITCHELL'').  Do not format title and section headings in all
capitals as well except for proper names (such as ``BLEU'') that are
conventionally in all capitals.  The affiliation should contain the
author's complete address, and if possible, an electronic mail
address. Start the body of the first page 7.5 cm from the top of the
page.

The title, author names and addresses should be completely identical
to those entered to the electronical paper submission website in order
to maintain the consistency of author information among all
publications of the conference. If they are different, the publication
chairs may resolve the difference without consulting with you; so it
is in your own interest to double-check that the information is
consistent.

{\bf Abstract}: Type the abstract at the beginning of the first
column. The width of the abstract text should be smaller than the
width of the columns for the text in the body of the paper by about
0.6 cm on each side. Center the word {\bf Abstract} in a 12 point bold
font above the body of the abstract. The abstract should be a concise
summary of the general thesis and conclusions of the paper. It should
be no longer than 200 words. The abstract text should be in 10 point font.

{\bf Text}: Begin typing the main body of the text immediately after
the abstract, observing the two-column format as shown in

the present document. Do not include page numbers.

{\bf Indent}: Indent when starting a new paragraph, about 0.4 cm. Use 11 points for text and subsection headings, 12 points for section headings and 15 points for the title.

\begin{table}
\centering
\small
\begin{tabular}{cc}
\begin{tabular}{|l|l|}
\hline
{\bf Command} & {\bf Output}\\\hline
\verb|{\"a}| & {\"a} \\
\verb|{\^e}| & {\^e} \\
\verb|{\`i}| & {\`i} \\ 
\verb|{\.I}| & {\.I} \\ 
\verb|{\o}| & {\o} \\
\verb|{\'u}| & {\'u}  \\ 
\verb|{\aa}| & {\aa}  \\\hline
\end{tabular} & 
\begin{tabular}{|l|l|}
\hline
{\bf Command} & {\bf  Output}\\\hline
\verb|{\c c}| & {\c c} \\ 
\verb|{\u g}| & {\u g} \\ 
\verb|{\l}| & {\l} \\ 
\verb|{\~n}| & {\~n} \\ 
\verb|{\H o}| & {\H o} \\ 
\verb|{\v r}| & {\v r} \\ 
\verb|{\ss}| & {\ss} \\\hline
\end{tabular}
\end{tabular}
\caption{Example commands for accented characters, to be used in, {\em e.g.}, \BibTeX\ names.}\label{tab:accents}
\end{table}

\subsection{Sections}

{\bf Headings}: Type and label section and subsection headings in the
style shown on the present document.  Use numbered sections (Arabic
numerals) in order to facilitate cross references. Number subsections
with the section number and the subsection number separated by a dot,
in Arabic numerals.
Do not number subsubsections.

\begin{table*}[t!]
\centering
\begin{tabular}{lll}
  output & natbib & previous \conforg{} style files\\
  \hline
  \citep{Gusfield:97} & \verb|\citep| & \verb|\cite| \\
  \citet{Gusfield:97} & \verb|\citet| & \verb|\newcite| \\
  \citeyearpar{Gusfield:97} & \verb|\citeyearpar| & \verb|\shortcite| \\
\end{tabular}
\caption{Citation commands supported by the style file.
  The citation style is based on the natbib package and
  supports all natbib citation commands.
  It also supports commands defined in previous \conforg{} style files
  for compatibility.
  }
\end{table*}

{\bf Citations}: Citations within the text appear in parentheses
as~\cite{Gusfield:97} or, if the author's name appears in the text
itself, as Gusfield~\shortcite{Gusfield:97}.
Using the provided \LaTeX\ style, the former is accomplished using
{\small\verb|\cite|} and the latter with {\small\verb|\shortcite|} or {\small\verb|\newcite|}. Collapse multiple citations as in~\cite{Gusfield:97,Aho:72}; this is accomplished with the provided style using commas within the {\small\verb|\cite|} command, {\em e.g.}, {\small\verb|\cite{Gusfield:97,Aho:72}|}. Append lowercase letters to the year in cases of ambiguities.  
 Treat double authors as
in~\cite{Aho:72}, but write as in~\cite{Chandra:81} when more than two
authors are involved. Collapse multiple citations as
in~\cite{Gusfield:97,Aho:72}. Also refrain from using full citations
as sentence constituents.

We suggest that instead of
\begin{quote}
  ``\cite{Gusfield:97} showed that ...''
\end{quote}
you use
\begin{quote}
``Gusfield \shortcite{Gusfield:97}   showed that ...''
\end{quote}

If you are using the provided \LaTeX{} and Bib\TeX{} style files, you
can use the command \verb|\citet| (cite in text)
to get ``author (year)'' citations.

If the Bib\TeX{} file contains DOI fields, the paper
title in the references section will appear as a hyperlink
to the DOI, using the hyperref \LaTeX{} package.
To disable the hyperref package, load the style file
with the \verb|nohyperref| option: \\{\small
\verb|\usepackage[nohyperref]{acl2018}|}

\textbf{Digital Object Identifiers}: As part of our work to make ACL
materials more widely used and cited outside of our discipline, ACL
has registered as a CrossRef member, as a registrant of Digital Object
Identifiers (DOIs), the standard for registering permanent URNs for
referencing scholarly materials. \conforg{} has \textbf{not} adopted the
ACL policy of requiring camera-ready references to contain the appropriate
  DOIs (or as a second resort, the hyperlinked ACL Anthology
  Identifier). But we certainly encourage you to use
  Bib\TeX\ records that contain DOI or URLs for any of the ACL
  materials that you reference. Appropriate records should be found
for most materials in the current ACL Anthology at
\url{http://aclanthology.info/}.

As examples, we cite \cite{P16-1001} to show you how papers with a DOI
will appear in the bibliography.  We cite \cite{C14-1001} to show how
papers without a DOI but with an ACL Anthology Identifier will appear
in the bibliography.  

\textbf{Anonymity:} As reviewing will be double-blind, the submitted
version of the papers should not include the authors' names and
affiliations. Furthermore, self-references that reveal the author's
identity, {\em e.g.},
\begin{quote}
``We previously showed \cite{Gusfield:97} ...''  
\end{quote}
should be avoided. Instead, use citations such as 
\begin{quote}
``\citeauthor{Gusfield:97} \shortcite{Gusfield:97}
previously showed ... ''
\end{quote}

Preprint servers such as arXiv.org and workshops that do not
have published proceedings are not considered archival for purposes of
submission. However, to preserve the spirit of blind review, authors
are encouraged to refrain from posting until the completion of the
review process. Otherwise, authors must state in the online submission
form the name of the workshop or preprint server and title of the
non-archival version. The submitted version should be suitably
anonymized and not contain references to the prior non-archival
version. Reviewers will be told: ``The author(s) have notified us that
there exists a non-archival previous version of this paper with
significantly overlapping text. We have approved submission under
these circumstances, but to preserve the spirit of blind review, the
current submission does not reference the non-archival version.''

\textbf{Please do not use anonymous citations} and do not include
 when submitting your papers. Papers that do not
conform to these requirements may be rejected without review.

\textbf{References}: Gather the full set of references together under
the heading {\bf References}; place the section before any Appendices,
unless they contain references. Arrange the references alphabetically
by first author, rather than by order of occurrence in the text.
By using a .bib file, as in this template, this will be automatically 
handled for you. See the \verb|\bibliography| commands near the end for more.

Provide as complete a citation as possible, using a consistent format,
such as the one for {\em Computational Linguistics\/} or the one in the 
{\em Publication Manual of the American 
Psychological Association\/}~\cite{APA:83}. Use of full names for
authors rather than initials is preferred. A list of abbreviations
for common computer science journals can be found in the ACM 
{\em Computing Reviews\/}~\cite{ACM:83}.

The \LaTeX{} and Bib\TeX{} style files provided roughly fit the
American Psychological Association format, allowing regular citations, 
short citations and multiple citations as described above.  

\begin{itemize}
\item Example citing an arxiv paper: \cite{rasooli-tetrault-2015}. 
\item Example article in journal citation: \cite{Ando2005}.
\item Example article in proceedings, with location: \cite{borsch2011}.
\item Example article in proceedings, without location: \cite{andrew2007scalable}.
\end{itemize}
See corresponding .bib file for further details.

Submissions should accurately reference prior and related work, including code and data. If a piece of prior work appeared in multiple venues, the version that appeared in a refereed, archival venue should be referenced. If multiple versions of a piece of prior work exist, the one used by the authors should be referenced. Authors should not rely on automated citation indices to provide accurate references for prior and related work.

{\bf Appendices}: Appendices, if any, directly follow the text and the
references (but see above).  Letter them in sequence and provide an
informative title: {\bf Appendix A. Title of Appendix}.

\subsection{URLs}

URLs can be typeset using the \verb|\url| command. However, very long
URLs cause a known issue in which the URL highlighting may incorrectly
cross pages or columns in the document. Please check carefully for
URLs too long to appear in the column, which we recommend you break,
shorten or place in footnotes. Be aware that actual URL should appear
in the text in human-readable format; neither internal nor external
hyperlinks will appear in the proceedings.

\subsection{Footnotes}

{\bf Footnotes}: Put footnotes at the bottom of the page and use 9
point font. They may be numbered or referred to by asterisks or other
symbols.\footnote{This is how a footnote should appear.} Footnotes
should be separated from the text by a line.\footnote{Note the line
separating the footnotes from the text.}

\subsection{Graphics}

{\bf Illustrations}: Place figures, tables, and photographs in the
paper near where they are first discussed, rather than at the end, if
possible.  Wide illustrations may run across both columns.  Color
illustrations are discouraged, unless you have verified that  
they will be understandable when printed in black ink.

{\bf Captions}: Provide a caption for every illustration; number each one
sequentially in the form:  ``Figure 1. Caption of the Figure.'' ``Table 1.
Caption of the Table.''  Type the captions of the figures and 
tables below the body, using 11 point text.

\subsection{Accessibility}
\label{ssec:accessibility}

In an effort to accommodate people who are color-blind (as well as those printing
to paper), grayscale readability for all accepted papers will be
encouraged.  Color is not forbidden, but authors should ensure that
tables and figures do not rely solely on color to convey critical
distinctions. A simple criterion: All curves and points in your figures should be clearly distinguishable without color.

% Min: no longer used as of ACL 2018, following ACL exec's decision to
% remove this extra workflow that was not executed much.
% BEGIN: remove
%% \section{XML conversion and supported \LaTeX\ packages}

%% Following ACL 2014 we will also we will attempt to automatically convert 
%% your \LaTeX\ source files to publish papers in machine-readable 
%% XML with semantic markup in the ACL Anthology, in addition to the 
%% traditional PDF format.  This will allow us to create, over the next 
%% few years, a growing corpus of scientific text for our own future research, 
%% and picks up on recent initiatives on converting ACL papers from earlier 
%% years to XML. 

%% We encourage you to submit a ZIP file of your \LaTeX\ sources along
%% with the camera-ready version of your paper. We will then convert them
%% to XML automatically, using the LaTeXML tool
%% (\url{http://dlmf.nist.gov/LaTeXML}). LaTeXML has \emph{bindings} for
%% a number of \LaTeX\ packages, including the ACL 2018 stylefile. These
%% bindings allow LaTeXML to render the commands from these packages
%% correctly in XML. For best results, we encourage you to use the
%% packages that are officially supported by LaTeXML, listed at
%% \url{http://dlmf.nist.gov/LaTeXML/manual/included.bindings}
% END: remove

\section{Translation of non-English Terms}

It is also advised to supplement non-English characters and terms
with appropriate transliterations and/or translations
since not all readers understand all such characters and terms.
Inline transliteration or translation can be represented in
the order of: original-form transliteration ``translation''.

\section{Length of Submission}
\label{sec:length}

The \confname{} main conference accepts submissions of long papers and
short papers.
 Long papers may consist of up to eight (8) pages of
content plus unlimited pages for references. Upon acceptance, final
versions of long papers will be given one additional page -- up to nine (9)
pages of content plus unlimited pages for references -- so that reviewers' comments
can be taken into account. Short papers may consist of up to four (4)
pages of content, plus unlimited pages for references. Upon
acceptance, short papers will be given five (5) pages in the
proceedings and unlimited pages for references. 

For both long and short papers, all illustrations and tables that are part
of the main text must be accommodated within these page limits, observing
the formatting instructions given in the present document. Supplementary
material in the form of appendices does not count towards the page limit; see appendix A for further information.

However, note that supplementary material should be supplementary
(rather than central) to the paper, and that reviewers may ignore
supplementary material when reviewing the paper (see Appendix
\ref{sec:supplemental}). Papers that do not conform to the specified
length and formatting requirements are subject to be rejected without
review.

Workshop chairs may have different rules for allowed length and
whether supplemental material is welcome. As always, the respective
call for papers is the authoritative source.

\section*{Acknowledgments}

The acknowledgments should go immediately before the references.  Do
not number the acknowledgments section. Do not include this section
when submitting your paper for review. \\

\noindent {\bf Preparing References:} \\

Include your own bib file like this:
{\small\verb|\bibliographystyle{acl_natbib_nourl}|
\verb|\bibliography{emnlp2018}|}

Where \verb|emnlp2018| corresponds to the {\tt emnlp2018.bib} file.
\bibliography{emnlp2018}
\bibliographystyle{acl_natbib_nourl}

\appendix

\section{Supplemental Material}
\label{sec:supplemental}
Each \confname{} submission can be accompanied by a single PDF
appendix, one {\small\tt.tgz} or {\small\tt.zip} appendix containing
software, and one {\small\tt.tgz} or {\small\tt.zip} appendix
containing data.

Submissions may include resources (software and/or data) used in in
the work and described in the paper. Papers that are submitted with
accompanying software and/or data may receive additional credit toward
the overall evaluation score, and the potential impact of the software
and data will be taken into account when making the
acceptance/rejection decisions. Any accompanying software and/or data
should include licenses and documentation of research review as
appropriate.

\confname{} also encourages the submission of supplementary material
to report preprocessing decisions, model parameters, and other details
necessary for the replication of the experiments reported in the
paper. Seemingly small preprocessing decisions can sometimes make a
large difference in performance, so it is crucial to record such
decisions to precisely characterize state-of-the-art methods.

Nonetheless, supplementary material should be supplementary (rather
than central) to the paper. {\bf Submissions that misuse the supplementary 
material may be rejected without review.}
Essentially, supplementary material may include explanations or details
of proofs or derivations that do not fit into the paper, lists of
features or feature templates, sample inputs and outputs for a system,
pseudo-code or source code, and data. (Source code and data should
be separate uploads, rather than part of the paper).

The paper should not rely on the supplementary material: while the paper
may refer to and cite the supplementary material and the supplementary material will be available to the
reviewers, they will not be asked to review the
supplementary material.

Appendices ({\em i.e.} supplementary material in the form of proofs, tables,
or pseudo-code) should be {\bf uploaded as supplementary material} when submitting the paper for review.
Upon acceptance, the appendices come after the references, as shown here. Use
\verb|\appendix| before any appendix section to switch the section
numbering over to letters.

\end{document}
